# Supplementary material for: A phase stable hybrid dual comb spectrometer
Source: arXiv:2211.05186 source file (2022-11-09)
Supplement: Supplementary file 1 [file supp_file.pdf]

# Supporting information:
# A phase stable hybrid dual comb spectrometer

Sutapa Ghosh and Gadi Eisenstein

*Andrew and Erna Viterby Department of Electrical Engineering and Russell Berrie Nanotechnology Institute, Technion-Israel Institute of Technology, Haifa 32000, Israel*

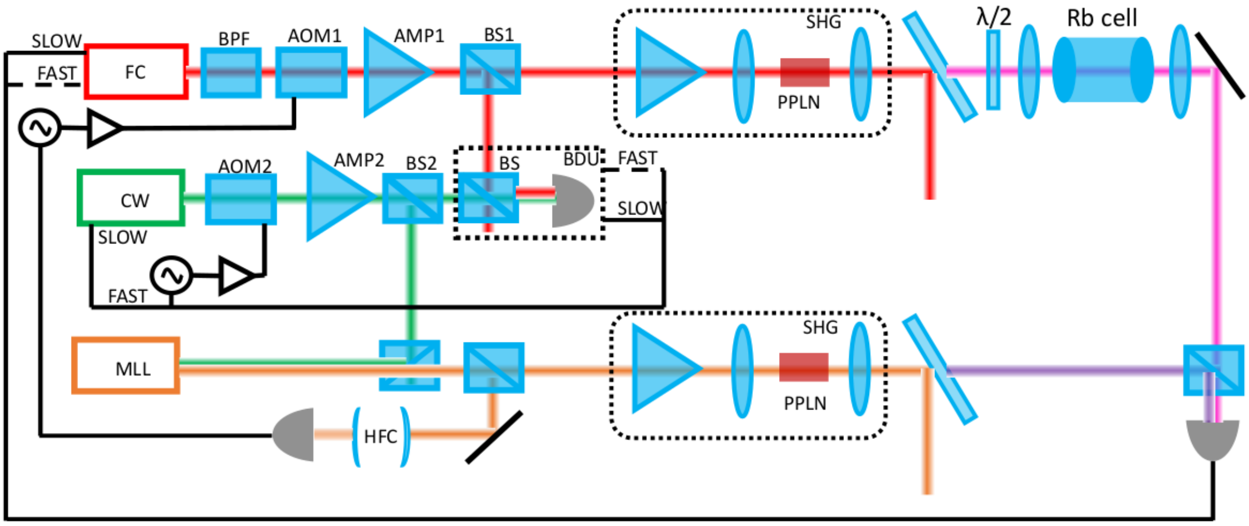


FIG. S1. **Detailed set-up of the hybrid dual comb spectroscopy.** A single line of a commercial FC is mixed with a CW laser. The resulting beat signal is used to stabilize the CW laser by fast feedback to AOM2 and slow feedback to the CW laser cavity. The CW laser injection locks the MLL. This transfers the fluctuations of the FC to the carrier envelop offset (CEO) of the MLL. The MLL is detected at the output of a high (360,000) finesse cavity (HFC) and an error signal is generated which provides feedback to AOM1 and to the FC cavity length. Both the FC and the MLL are amplified and frequency doubled by periodically poled lithium niobate crystals (PPLN). The frequency doubled FC interrogates the rubidium cell and is combined with the second harmonic of the MLL to generate the RF beats.

## I. DETAILED EXPERIMENTAL SET UP

The schematics of the detailed experimental set up is shown in Fig. S1.

## II. CALCULATION OF THE ERROR SIGNAL OF A BROADBAND LASER

In this section, we generalize the theory of modulation spectroscopy for a comb field. Due to the broadband comb spectrum, many comb lines are resonant with the cavity and thus contribute to the error signal, which leads to stabilization of the entire comb spectrum.

Consider a frequency comb field with a repetition rate, $\omega_{rep}$ and carrier-envelope offset, $\omega_{ceo}$. The electric field can be written as:

$$E_{in} = \sum_{l=-\infty}^{\infty} A_l e^{-i\omega_l t} + \text{h.c.}$$

where, $\omega_l = l\omega_{rep} + \omega_{ceo}$ and $\omega_l$ is the carrier frequency.

The comb field is modulated at a frequency, $\Omega$ with a modulation depth, $\beta$.

$$
\begin{aligned}
E_{\mathrm{mod}} &= \sum_{l=-\infty}^{\infty} A_l e^{-i(\omega_l t+\beta \sin \Omega t)} + \text{h.c.} \\
&= \sum_l A_l e^{-i\omega_l t}[J_0(\beta) + 2\sum_{n=1}^{\infty} J_{2n}(\beta)\cos 2n\Omega t + 2i\sum_{n=0}^{\infty} J_{2n+1}(\beta)\sin{(2n+1)\Omega t}] \\
&= \sum_l A_l e^{-i\omega_l t}[J_0(\beta) + \sum_{n=1}^{\infty} J_{2n}(\beta)(e^{i2n\Omega t} + e^{-i2n\Omega t}) + \sum_{n=0}^{\infty} J_{2n+1}(e^{i(2n+1)\Omega t} + e^{-i(2n+1)\Omega t})] \\
&= \sum_l A_l [J_0(\beta)e^{-i\omega_l t} + \sum_{n=1}^{\infty} J_n(\beta)(e^{-i(\omega_l - n\Omega)t} + (-1)^n e^{-i(\omega_l+n\Omega)})]
\end{aligned}
$$

After the light passes through the cavity, the electric field of each comb line is modified by the corresponding cavity transfer function,

$$
E_{cav} = \sum_l A_l[J_0(\beta)T_l(\omega_l)e^{-i\omega_l t} + \sum_{n=1}^{\infty} J_n(\beta)T_l(\omega_l - n\Omega)e^{-i(\omega_l - n\Omega)t} + (-1)^n J_n(\beta)T(\omega_l + n\Omega)e^{-i(\omega_l+n\Omega)}]
$$

The cavity transfer function corresponding to the comb line $l$ is, $T_l(\omega)$ is given by,

$$
T_l(\omega) = \frac{\kappa_{cav}(\kappa_{cav} - i(\omega - \omega_{cav,l}))}{(\omega - \omega_{cav,l})^2 + \kappa_{cav}^2}
$$

where, $\kappa_{cav}$ represents the linewidth of the cavity mode, $\omega_{cav}$. The photo-detected signal becomes:

$$
\begin{aligned}
P_{error} = \sum_l |A_l|^2[&\text{dc terms} + \sum_{n=1}^{\infty} J_0(\beta)J_n(\beta)(T_l(\omega_l)T_l^*(\omega_l - n\Omega)e^{-in\Omega t} + T_l^*(\omega_l)T_l(\omega_l - n\Omega)e^{in\Omega t}) + \\
&(-1)^n(T_l(\omega_l)T_l^*(\omega_l + n\Omega)e^{in\Omega t} + T_l^*(\omega_l)T_l(\omega_l + n\Omega)e^{-in\Omega t}) + \sum_{n=1}^{\infty}\sum_{m=1}^{\infty} J_n(\beta)J_m(\beta) \\
&(T_l(\omega_l - n\Omega)T_l^*(\omega_l - m\Omega)e^{i(n-m)\Omega t} + T_l^*(\omega_l - n\Omega)T_l(\omega_l - m\Omega)e^{-i(n-m)\Omega t} + \\
&(-1)^{n+m}T_l(\omega_l + n\Omega)T_l^*(\omega_l + m\Omega)e^{-i(n-m)\Omega t} + (-1)^{n+m}T_l^*(\omega_l + n\Omega)T_l(\omega_l + m\Omega)e^{i(n-m)\Omega t})] + \text{higher orders}
\end{aligned}
$$

The frequency component, $e^{\pm i\Omega t}$, is filtered out and constitutes the error signal for the laser lock.

$$
\begin{aligned}
P_{error} = \sum_l A_l[&\text{dc term} + J_0(\beta)J_1(\beta)\text{Re}\{T_l(\omega_l)T_l^*(\omega_l - \Omega) - T_l(\omega_l + n\Omega)T^*(\omega_l)\} + \text{Im}\{T_l(\omega_l)T_l^*(\omega_l - \Omega) - \\
&T_l(\omega_l + n\Omega)T^*(\omega_l)\} + \sum_{n\neq m}\sum_{m=n-1}^{n+1} J_n(\beta)J_m(\beta)\text{Re}\{T_l(\omega_l - n\Omega)T_l^*(\omega_l - m\Omega) - T_l^*(\omega_l + n\Omega)T_l(\omega_l + n\Omega)\} + \\
&\text{Im}\{T_l(\omega_l - n\Omega)T_l^*(\omega_l - m\Omega) - T_l^*(\omega_l + n\Omega)T_l(\omega_l + n\Omega)\}]
\end{aligned}
$$

To obtain the optimum error signal in the experiment, we calculated the error with a high signal-to-noise ratio with respect to the modulation depth and frequency shown in Fig. 2 (b).
